# Supplementary material for: Discovery of ST1 centers in natural diamond
Source: arXiv:1906.04385 source file (2019-06-20)
Supplement: Supplementary file 1 [file top-matter-appendix.tex]

% \journalname{Nanophotonics}

% \author[2,3,*]{Priyadharshini ~Balasubramanian$^\dagger$}
% \author[2,3,*]{Mathias~H.~Metsch$^\dagger$}
% \author[1,*]{Prithvi~Reddy$^\dagger$}
% \author[4,5]{Lachlan~J.~Rogers}
% \author[1]{Neil~B.~Manson}
\author[]{}
% \author[2,3]{Fedor~Jelezko}

% \affil[*] {
%     These authors contributed equally to this work.
% }

% \affil[1]{%
%     Laser Physics Centre, Research School of Physics and Engineering, Australian National University, Acton, 2601, Australia
% }
% \affil[2]{%
%     Institute for Quantum Optics, University Ulm, Albert-Einstein-Allee 11, D-89081 Ulm, Germany
% }%
% \affil[3]{%
%     Center for Integrated Quantum Science and Technology (IQST), University Ulm, Albert-Einstein-Allee 11, D-89081 Ulm, Germany
% }%
% \affil[4]{
%     Department of Physics and Astronomy, Macquarie University, New South Wales 2109, Australia
% }
% \affil[5]{
%     ARC Centre of Excellence for Engineered Quantum Systems (EQUS)
% }
